# Supplementary material for: Learning Varying Physical Therapist-Patient Interactions for Robot-mediated Upper Limb Task-Specific Training
Source: arXiv:2608.15995 source file (2026-08-17)
Supplement: Supplementary file 1 [file 6_appendix.tex]

\appendices

\section*{Acknowledgment}
I want to acknowledge the fact that this thing is hard to do.

\section{Submitting Your Paper for Review}
\section{IEEE Publishing Policy}
\section{Publication Principles}

% \section*{Possible Approaches When Persistent Excitation Is Not Satisfied in TP-GMM}
 
% In many Learning from Demonstration (LfD) problems, and particularly in Task-Parameterized Gaussian Mixture Models (TP-GMM), the demonstrations do not satisfy a classical persistent excitation (PE) condition. Consequently, unique parameter identification cannot be guaranteed.
 
% Rather than attempting to recover the ``true'' parameters, the goal should be to obtain a model that reproduces the demonstrated skill accurately and generalizes well to unseen task configurations.
 
% The following approaches can be explored.
 
% \subsection*{1. Reduce Model Complexity}
 
% An over-parameterized TP-GMM often suffers from poor generalization.
 
% Possible actions include:
% \begin{itemize}
%     \item Reducing the number of Gaussian components.
%     \item Simplifying covariance structures.
%     \item Removing unnecessary parameters.
% \end{itemize}
 
% For example, compare
 
% \[
% K = 3,4,5
% \]
 
% against
 
% \[
% K = 10,15,20.
% \]
 
% A smaller model may provide better generalization.
 
% \subsection*{2. Covariance Regularization}
 
% To avoid ill-conditioned covariance estimates, replace
 
% \[
% \Sigma_k
% \]
 
% with
 
% \[
% \Sigma_k + \lambda I,
% \]
 
% where $\lambda > 0$ is a regularization parameter.
 
% This improves numerical robustness and prevents covariance collapse.
 
% \subsection*{3. Remove Redundant Task Frames}
 
% TP-GMM performance may degrade when multiple task frames provide similar information.
 
% A useful experiment is to:
% \begin{enumerate}
%     \item Remove one task frame.
%     \item Retrain the model.
%     \item Compare reproduction performance.
% \end{enumerate}
 
% Frames that contribute little to performance may be redundant.
 
% \subsection*{4. Cross-Validation}
 
% Evaluate generalization using:
% \begin{itemize}
%     \item Leave-one-demonstration-out validation.
%     \item Leave-one-task-configuration-out validation.
% \end{itemize}
 
% Performance metrics may include:
 
% \[
% \text{RMSE},
% \qquad
% \text{tracking error},
% \qquad
% \text{reproduction accuracy}.
% \]
 
% \subsection*{5. Collect More Diverse Demonstrations}
 
% Instead of collecting additional demonstrations of the same task, increase task diversity by varying:
 
% \begin{itemize}
%     \item Initial positions,
%     \item Goal positions,
%     \item Object orientations,
%     \item Object locations,
%     \item Execution speeds.
% \end{itemize}
 
% This is the closest practical analogue to increasing excitation.
 
% \subsection*{6. Data Augmentation}
 
% Artificial demonstrations can be generated through:
 
% \begin{itemize}
%     \item Rotations,
%     \item Translations,
%     \item Scaling,
%     \item Time warping.
% \end{itemize}
 
% This increases coverage of the task space without collecting additional demonstrations.
 
% \subsection*{7. Deliberate Perturbation Demonstrations}
 
% Ask the demonstrator to intentionally vary:
 
% \begin{itemize}
%     \item Approach angles,
%     \item Speeds,
%     \item Path shapes,
%     \item Intermediate waypoints.
% \end{itemize}
 
% Such variations can reveal task dependencies that remain hidden in highly repetitive demonstrations.
 
% \subsection*{8. Sensitivity Analysis}
 
% Evaluate parameter influence by perturbing each parameter:
 
% \[
% \theta_i \rightarrow \theta_i + \delta.
% \]
 
% Measure the resulting trajectory change
 
% \[
% \Delta y.
% \]
 
% Parameters that produce negligible changes may be removed.
 
% \subsection*{9. Singular Value Analysis}
 
% Construct a sensitivity matrix
 
% \[
% J
% =
% \frac{\partial y}{\partial \theta}.
% \]
 
% Compute its singular value decomposition
 
% \[
% J = U \Sigma V^T.
% \]
 
% Small singular values indicate poorly identifiable parameter directions.
 
% This provides a practical diagnostic of parameter redundancy.
 
% \subsection*{10. Frame Relevance Analysis}
 
% For each task frame:
 
% \begin{enumerate}
%     \item Remove the frame.
%     \item Retrain TP-GMM.
%     \item Evaluate reproduction quality.
% \end{enumerate}
 
% If performance remains unchanged, the frame may not contribute useful information.
 
% \subsection*{11. Bayesian TP-GMM}
 
% Treat model parameters as random variables:
 
% \[
% \theta \sim p(\theta).
% \]
 
% Posterior uncertainty can be used to assess parameter confidence.
 
% Large posterior variances suggest insufficient information in the demonstrations.
 
% \subsection*{12. Sparse Learning}
 
% Introduce sparsity-promoting regularization:
 
% \[
% \min_{\theta}
% \;
% J(\theta)
% +
% \lambda \|\theta\|_1.
% \]
 
% This automatically suppresses weakly supported parameters.
 
% \subsection*{13. Latent-Space TP-GMM}
 
% Apply dimensionality reduction before learning:
 
% \begin{itemize}
%     \item Principal Component Analysis (PCA),
%     \item Autoencoders,
%     \item Variational Autoencoders (VAE).
% \end{itemize}
 
% TP-GMM is then learned in a lower-dimensional latent space, reducing the identification burden.
 
% \subsection*{14. Define a Task Excitation Metric}
 
% A possible research direction is to define an analogue of persistent excitation for TP-GMM.
 
% Let
 
% \[
% z_i
% \]
 
% represent the task-parameter vector associated with demonstration $i$.
 
% Define
 
% \[
% E
% =
% \lambda_{\min}
% \left(
% \sum_{i=1}^{N}
% z_i z_i^T
% \right).
% \]
 
% Larger values of $E$ indicate richer task variation.
 
% The relationship between $E$ and generalization performance can then be investigated.
 
% \subsection*{15. Active Demonstration Selection}
 
% Instead of collecting demonstrations randomly, select demonstrations that maximize information gain.
 
% Possible criteria include
 
% \[
% \max \det(F),
% \]
 
% where $F$ denotes a Fisher information matrix or an uncertainty measure.
 
% This connects Learning from Demonstration with optimal experiment design.
 
% \section*{Recommended Initial Experiments}
 
% Before pursuing theoretical analyses, the following experiments are recommended:
 
% \begin{enumerate}
%     \item Vary the number of Gaussian components.
%     \item Add covariance regularization.
%     \item Remove task frames one at a time.
%     \item Perform sensitivity and singular value analysis.
%     \item Collect a small set of deliberately diverse demonstrations.
% \end{enumerate}
 
% These experiments often reveal the main limitations of the dataset and model more effectively than attempting to verify a persistent excitation condition.
